# Supplementary material for: Modeling the [Fe II]{\lambda}1.644{\mu}m outflow and comparison with H$_2$ and H$^+$ kinematics in the inner 200 pc of NGC 1068
Source: arXiv:1408.4750 source file (2014-08-20)
Supplement: Supplementary file 1 [file p-appendix-only.pdf]

Appendix to the paper:  
Modeling the [Fe II] $\lambda$  1.644 $\mu$ m outflow and comparison with  
H<sub>2</sub> and H<sup>+</sup> kinematics in the inner 200 pc of NGC 1068

F. K. B. Barbosa<sup>1\*</sup>, T. Storchi-Bergmann<sup>2</sup>, P. McGregor<sup>3</sup> and T. B. Vale<sup>4</sup>

<sup>1</sup>IFRS – Campus Restinga, Rua 7121, n. 285 Lote 16, Quadra F, Restinga, CEP 91791-508, Porto Alegre, RS, Brazil

<sup>2</sup>Instituto de Física – UFRGS, Caixa Postal 15051, CEP 91501-970, Porto Alegre, RS, Brazil

<sup>3</sup>Research School of Astronomy and Astrophysics, Australian National University, Cotter Road, Weston Creek, ACT 2611, Australia

<sup>4</sup>INFES – UFF, Rua João Jasbick, s/n, Bairro Aeroporto, CEP 28470-000 Santo Antônio de Pádua, RJ, Brazil

30 july 2014

---

\*E-mail: fausto.barbosa@restinga.ifrs.edu.br

## A Conical outflow model figures

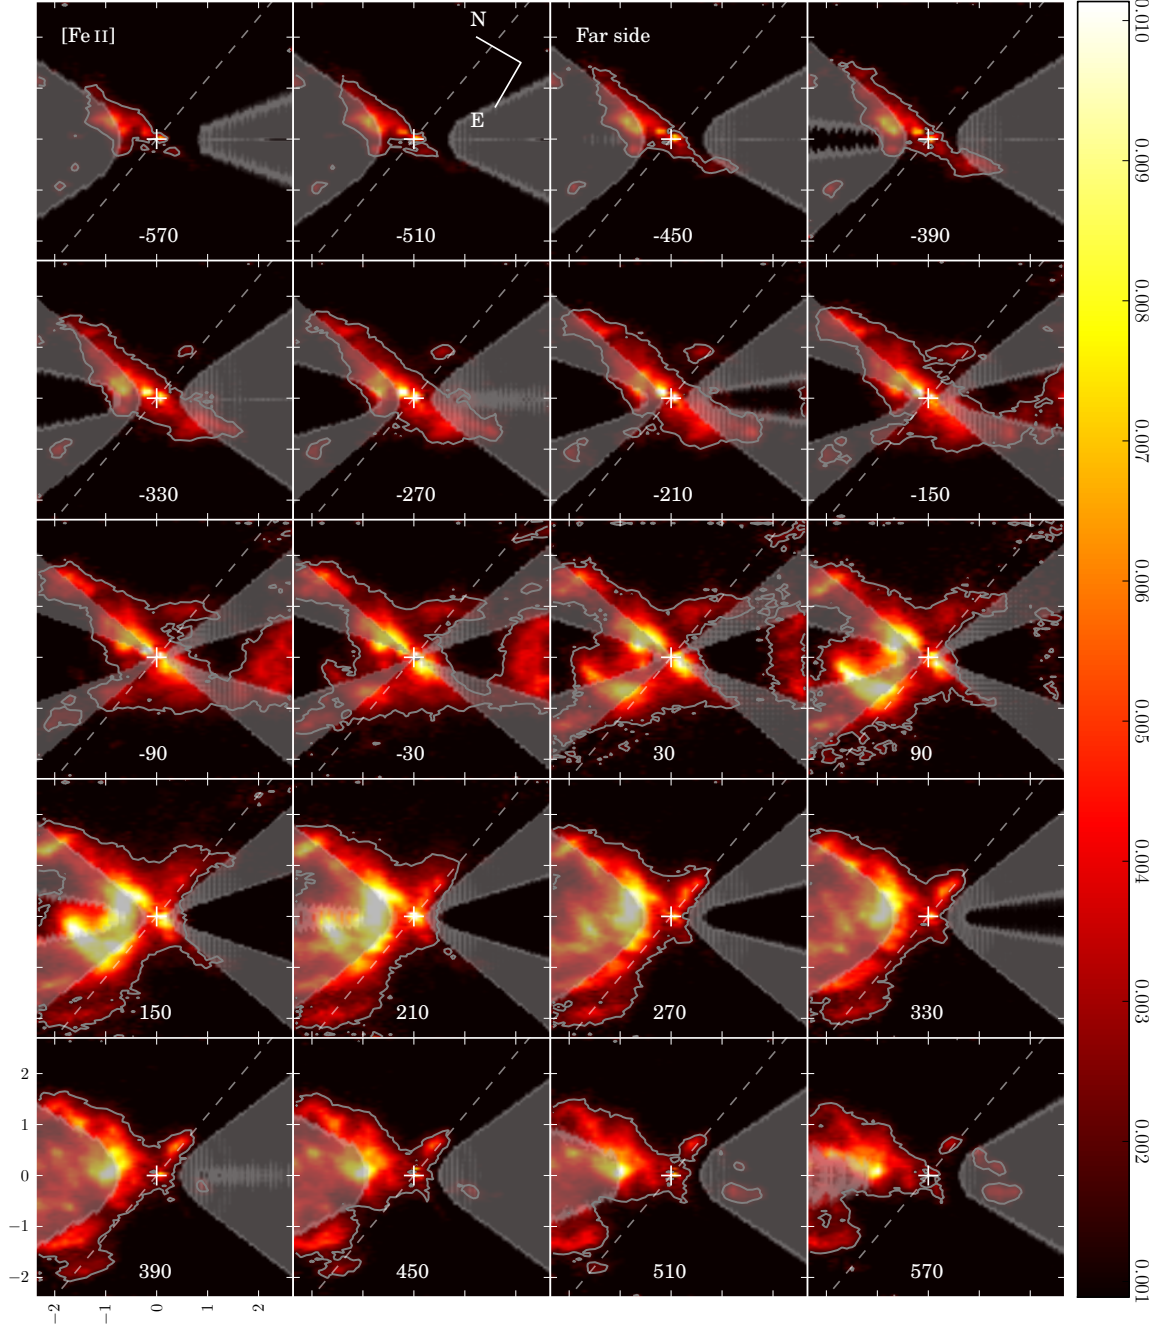

Figure 1: Channel maps of the accelerated conical outflow model for the [Fe II] line (grey levels) superimposed to the data (hot colours). The data was interpolated in wavelength to the same velocity range as the model. The central velocity of each channel is displayed in  $\text{km s}^{-1}$  at the bottom of the corresponding panel. The dashed line is the adopted major axis of the galaxy. The tick labels are given in arcsec in the lower left panel. The orientation and adopted far side are indicated in the upper panels.

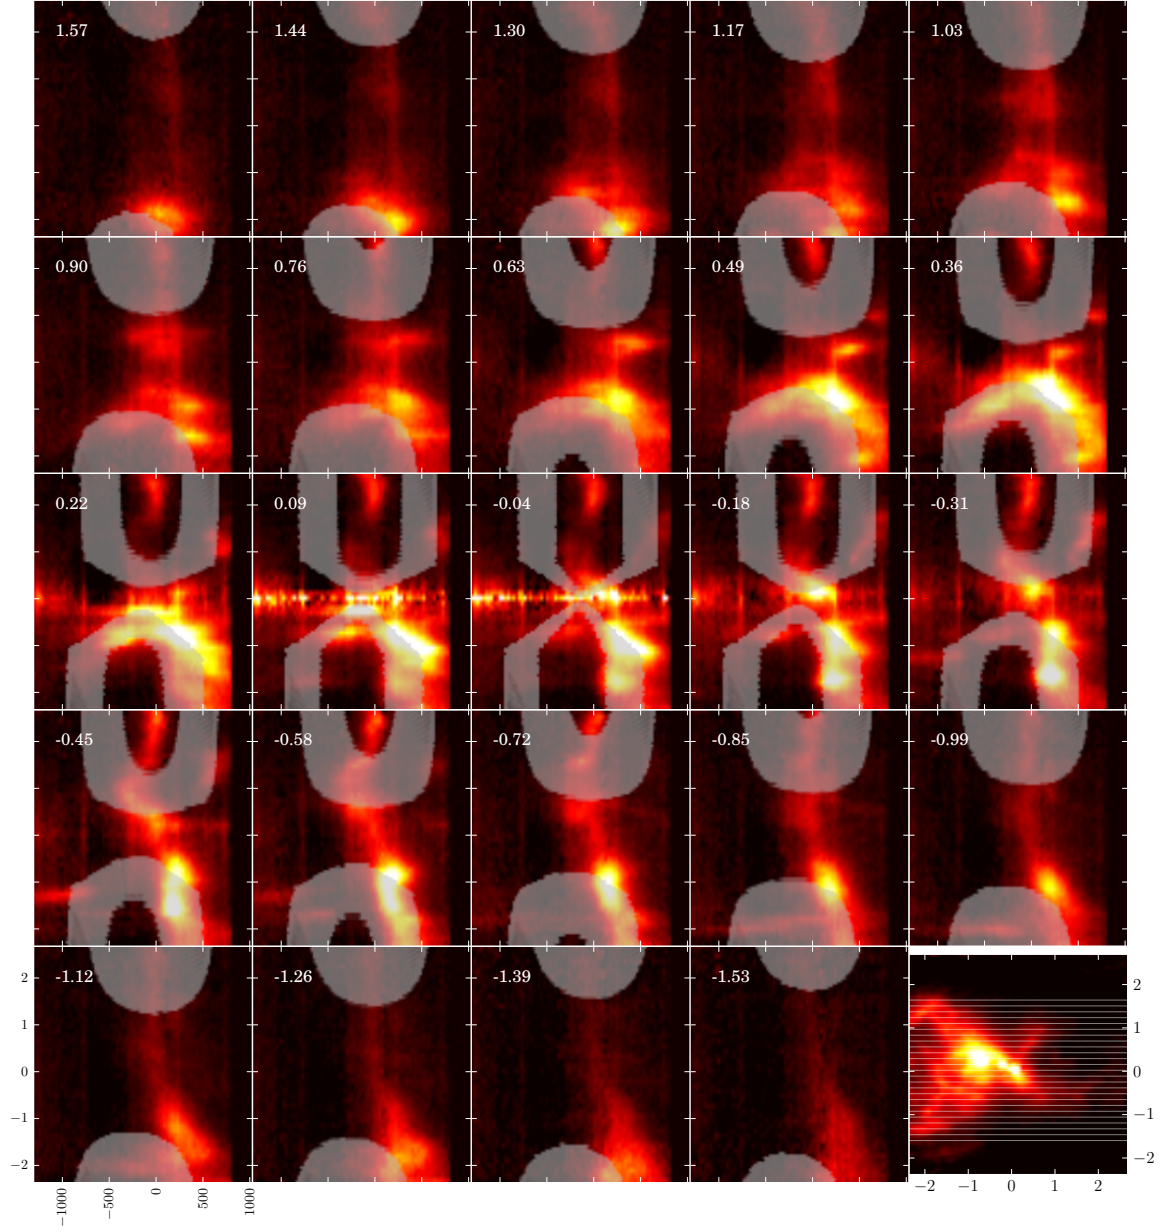

Figure 2: Position-velocity diagrams of the accelerated conical outflow model for the [Fe II] line (grey levels) superimposed to the data (hot colours). In the lower right panel of the figure we draw the integrated flux map (hot colours) and the lines corresponding to the limits of the adopted slits. The vertical displacement from the nucleus to the center of each slit is displayed in the upper left corner of each panel, in arcsec.

## B Spherical outflow model figures

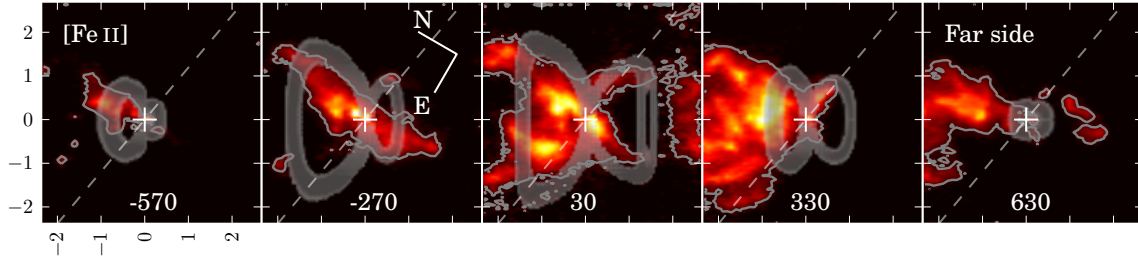

Figure 3: Channel maps of the spherical outflow model for the [Fe II] line (grey levels) superimposed to the data (hot colours). The data was interpolated in wavelength to the same velocity range as the model. The central velocity of each channel is displayed in  $\text{km s}^{-1}$  at the bottom of the corresponding panel. The dashed line is the adopted major axis of the galaxy. The tick labels are given in arcsec in the left panel, the orientation is indicated in the panel with  $v = -270 \text{ km s}^{-1}$  and the adopted far side is indicated in the right panel.

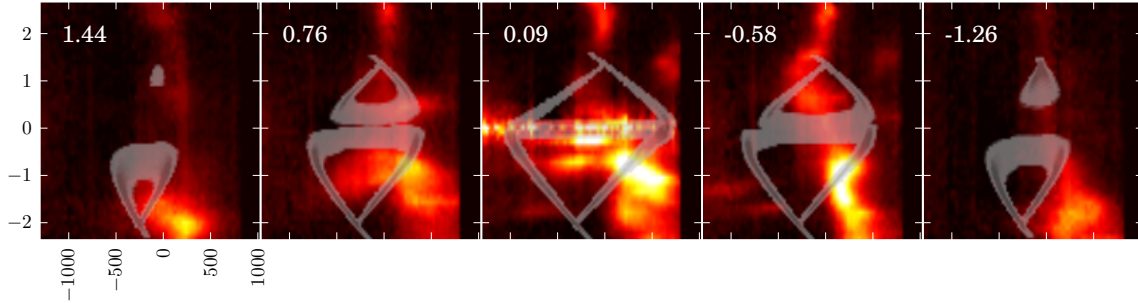

Figure 4: Position-velocity diagrams of the spherical outflow model for the [Fe II] line (grey levels) superimposed to the data (hot colours). The vertical displacement from the nucleus to the center of each slit is displayed in the upper left corner of each panel, in arcsec.
